# Supplementary material for: Continuously updated estimation of conditional hazard functions
Source: arXiv:2503.08356 source file (2025-07-02)
Supplement: Supplementary file 1 [file hazard_SM.pdf]

# Continuously updated approach to estimating conditional hazard functions *Supplementary Material*

Daphné Aurouet* Valentin Patilea†

March 11, 2025

**Abstract**

In this supplement we provide details of the construction of the simulation design, additional simulation results, and some technical proofs.

## 1 Details on the construction of the simulation design

The setup for the simulation experiment was designed to match the Rotterdam primary breast cancer data set containing 2982 patients, as considered by Royston and Altman (2013); see also Foekens et al. (2000). The event of interest is the occurrence of death from breast cancer after a surgery.

### 1.1 Simulation design

Recall that we considered two models for generating the time-to-event $T$: 'Model 1' based on Cox's Proportional Hazard (CPH) model, see Cox (1972); and 'Model 2' using the Accelerated Failure Time (AFT) model, see Wei (1992). Thus, the conditional hazard functions given $\mathbf{X} = \boldsymbol{x}$ are defined as

$$\lambda_{T|\mathbf{X}}(t \mid \boldsymbol{x}) = \lambda_0(t)\exp(\boldsymbol{x}^\top\boldsymbol{\beta}) \quad \text{and} \quad \lambda_{T|\mathbf{X}}(t \mid \boldsymbol{x}) = \lambda_0(t\exp(\boldsymbol{x}^\top\boldsymbol{\beta}))\exp(\boldsymbol{x}^\top\boldsymbol{\beta}),$$

*Ensai, CREST - UMR 9194, France; daphne.aurouet@ensai.fr

†Corresponding authors: Ensai, CREST - UMR 9194, France; valentin.patilea@ensai.fr

respectively. Here, for any vector $\boldsymbol{a}$, $\boldsymbol{a}^\top$ denotes its transpose. The expression of the baseline hazard $\lambda_0(t)$ is

$$\lambda_0(t) = \alpha_1 + \alpha_2 t + \alpha_3 t^2 + \alpha_4 \exp(\alpha_5 t).$$

To generate a time-to-event $T$ starting from the conditional hazard function given $\mathbf{X} = \boldsymbol{x}$, we first compute the conditional survival function as the exponential of the conditional integrated hazard function, and next use the inverse transform sampling method.

The vector of model coefficients $\boldsymbol{\beta}$ as well as the vector $\boldsymbol{\alpha} = (\alpha_1, \ldots, \alpha_5)^\top$ are set to match the estimates obtained with the CPH when fitted to the Rotterdam breast cancer data. More precisely, we consider as covariates the standardized age of the patient and the number of positive lymph nodes, while the binary variables are the size of the tumor (small, medium or large, the latter being the reference) and the report of a relapse. The coefficients $\boldsymbol{\beta}$ are estimated using the `R` package `survival`. To set our baseline hazard function parameters $\boldsymbol{\alpha}$, we fit by nonlinear least squares $\lambda_0(\cdot)$ to a hazard function calculated with the Rotterdam breast cancer data. The latter is obtained by finite differences from Breslow (1972)'s estimator of the baseline cumulative hazard function. This preliminary step for defining the simulation design leads us to consider Model 1 with

$$\boldsymbol{\beta}_{\text{CPH}} = (0.24, 0.04, -0.69, -0.32, 1.9)^\top \quad \text{and} \quad \boldsymbol{\alpha} = (-20.32, -1.51, -0.08, 20.32, 0.08)^\top.$$

For Model 2, we set $\boldsymbol{\beta}_{\text{AFT}} = \boldsymbol{\beta}_{\text{CPH}}/4$, which makes the hazard functions for the two models to have comparable scales. Finally, the censoring times $C$ are drawn from an exponential law of parameter 0.45 and shifted by a constant $\mu_C$. The constant is adjusted to allow for various censoring schemes such that $\mu_C \in \{8.3, 6.5, 3.5\}$ for 20%, 40%, and 60%, respectively for Model 1 and $\mu_C \in \{8.25, 6, 4.5\}$ for Model 2.

We define our covariate vector $\mathbf{X}$ as follows. One continuous variable, named $\mathbf{X}_{c,1}$, is a proxy of the standardized patient's age at the surgery. It is considered to be supported on $[-3, 3]$ with the same distribution as the variable $3A-6$ where $A$ is generated from a mixture of two Beta distributions $\pi\mathcal{B}(a_1, b_1) + (1-\pi)\mathcal{B}(a_2, b_2)$, with parameters $a_1 = 17, b_1 = 10$, $a_2 = 9, b_2 = 14$ and $\pi = 0.4$. These parameters were selected such that the Beta mixture density matches the kernel estimate of the standardized age from the real data set. A second continuous variable, named $\mathbf{X}_{c,2}$, has a Gamma distribution with the parameters selected to fit the sample mean and variance of the number of lymph nodes, that are $(0.38, 0.14)$, which means the expectation is approximately 2.709. The vector $\mathbf{X}$ is completed by three binary covariates obtained from a multinomial variable with parameters $(0.47, 0.1, 0.43)$, which is a proxy for the tumor variable, and a Bernoulli variable with parameter $(0.51)$, accounting for the presence of a relapse.

## 1.2 Additional simulation results

Below we compare our RCH estimator of the conditional hazard with that of the semi-parametric Cox's Proportional Hazard model fitted using the `R` package `survival`, called CPH estimator in the following. Given the estimate of $\boldsymbol{\beta}$ by maximization of Cox's partial likelihood, the CPH estimate of the conditional hazard function is derived from Breslow's estimate (see Breslow (1972)) by finite differences, which are eventually smoothed by splines. Since Model 1 is a proportional hazard model, we use the CPH estimator as benchmark for both models.

Table 1 complete the results reported in Figure 1 from the manuscript, and show the simulation results when the data are generated according to Model 1 and Model 2. As expected, the CPH estimator performs better in Model 1 which is a Cox's PH setup. The errors deteriorate as the sample size increasing because the CPH estimator has a parametric rate of convergence. In the AFT setup our nonparametric approach remains consistent and eventually outperforms the CPH estimator which is not consistent.

Table 1: Median of the MISE over 500 replications for different models, censoring rates, and sample sizes.

| model | censoring | estimator | 200 | 400 | 1000 | 2000 | 5000 | 10000 | 20000 |
|---|---|---|---|---|---|---|---|---|---|
| Model 1 | 20% | RCH | 0.0176 | 0.0127 | 0.0078 | 0.0053 | 0.0033 | 0.0023 | 0.0017 |
| | | CPH | 0.0024 | 0.0012 | 0.0005 | 0.0003 | 0.0001 | 0.0001 | 0.0001 |
| | 40% | RCH | 0.0156 | 0.0112 | 0.0067 | 0.0045 | 0.0027 | 0.0019 | 0.0014 |
| | | CPH | 0.0027 | 0.0013 | 0.0005 | 0.0003 | 0.0001 | 0.0001 | 0.0001 |
| | 60% | RCH | 0.0115 | 0.0080 | 0.0048 | 0.0032 | 0.0020 | 0.0014 | 0.0011 |
| | | CPH | 0.0033 | 0.0016 | 0.0007 | 0.0003 | 0.0001 | 0.0001 | 0.0001 |
| Model 2 | 20% | RCH | 0.0501 | 0.0402 | 0.0253 | 0.0145 | 0.0063 | 0.0044 | 0.0042 |
| | | CPH | 0.0130 | 0.0111 | 0.0104 | 0.0101 | 0.0099 | 0.0098 | 0.0097 |
| | 40% | RCH | 0.0286 | 0.0236 | 0.0154 | 0.0096 | 0.0041 | 0.0027 | 0.0027 |
| | | CPH | 0.0104 | 0.0095 | 0.0082 | 0.0077 | 0.0076 | 0.0075 | 0.0076 |
| | 60% | RCH | 0.0165 | 0.0144 | 0.0108 | 0.0078 | 0.0041 | 0.0023 | 0.0015 |
| | | CPH | 0.0083 | 0.0069 | 0.0063 | 0.0060 | 0.0060 | 0.0059 | 0.0058 |

# 2 Technical details

The following lemma was stated in the manuscript. Here, we also provide the proof.

**Lemma 1.** *Let $\rho \geq 0$, $\varrho > 0$, $\varrho \neq 1$, and $n > 1$. Then*

$$\frac{(n+1)^{1-\varrho}}{1-\varrho} - \frac{1}{1-\varrho} \leq \sum_{i=1}^{n} i^{-\varrho} \leq \frac{n^{1-\varrho}}{1-\varrho} - \frac{\varrho}{1-\varrho}, \tag{1}$$

*and*

$$\frac{n^{1+\rho}}{1+\rho}+\frac{\rho}{1+\rho}\leq\sum_{i=1}^{n}i^{\rho}\leq\frac{(n+1)^{1+\rho}}{1+\rho}-\frac{1}{1+\rho},\tag{2}$$

*Proof of Lemma 1.* For any $i \geq 1$ and $x \in [i, i+1]$, we have

$$(i+1)^{-\varrho}\leq x^{-\varrho}\leq i^{-\varrho}.$$

We then deduce

$$\sum_{i=2}^{n+1}i^{-\varrho}=\sum_{i=1}^{n}(i+1)^{-\varrho}\leq\int_{1}^{n+1}x^{-\varrho}dx=\frac{1}{1-\varrho}\left[(n+1)^{1-\varrho}-1\right]\leq\sum_{i=1}^{n}i^{-\varrho},$$

from which (1) above follows.

Since $\rho > 0$, for any $i \geq 1$ and $x \in [i, i+1]$, we have $i^{\rho} \leq x^{\rho} \leq (i+1)^{\rho}$, and thus

$$\sum_{i=1}^{n}i^{\rho}\leq\int_{1}^{n+1}x^{\rho}dx=\frac{1}{1+\rho}\left[(n+1)^{1+\rho}-1\right]\leq\sum_{i=1}^{n}(i+1)^{\rho}=\sum_{i=2}^{n+1}i^{\rho},$$

and (2) above follows. The case $\rho = 0$ is obvious. □

# References


Breslow, N. E. (1972). Contribution to discussion of paper by D. R. Cox. *J. Roy. Statist. Soc. Ser. B*, 34:216–217.

Cox, D. R. (1972). Regression models and life-tables. *J. Roy. Statist. Soc. Ser. B*, 34:187–220.

Foekens, J. A., Peters, H. A., Look, M. P., Portengen, H., Schmitt, M., Kramer, M. D., Brünner, N., Jänicke, F., Gelder, M. E. M.-v., Henzen-Logmans, S. C., et al. (2000). The urokinase system of plasminogen activation and prognosis in 2780 breast cancer patients. *Cancer research*, 60(3):636–643.

Royston, P. and Altman, D. G. (2013). External validation of a Cox prognostic model: principles and methods. *BMC medical research methodology*, 13:1–15.

Wei, L.-J. (1992). The accelerated failure time model: a useful alternative to the Cox regression model in survival analysis. *Statistics in Medicine*, 11(14-15):1871–1879.
